# Supplementary material for: DynE: Dynamic Ensemble Decoding for Multi-Document Summarization
Source: arXiv:2006.08748 source file (2020-06-15)
Supplement: Supplementary file 1 [file 7-appendix.tex]

\subsection{Notes on Rouge Evaluation}

Recent work uses several different workflows for evaluating Rouge. Here we present full results with evaluation scripts from \citet{ghalandari2020WCEP}, \citet{lebanoff-etal-2018-adapting}, and \citet{multinews2019}\footnote{All evaluation code available at \url{https://github.com/chrishokamp/dynamic-transformer-ensembles}}.
